# Supplementary material for: Verifiable Access Control for Augmented Reality Localization and Mapping
Source: arXiv:2203.13308 source file (2022-03-24)
Supplement: Supplementary file 1 [file 10-appendix.tex]

\section{Appendix}

\fixme{If time permits, define the privacy policies for each basic scenario.}
